# Supplementary material for: Conditioning Trick for Training Stable GANs
Source: arXiv:2010.05844 source file (2020-10-12)
Supplement: Supplementary file 1 [file supplementary.tex]

\documentclass{article} % For LaTeX2e
\usepackage{iclr2021_conference,times}

% Optional math commands from https://github.com/goodfeli/dlbook_notation.
\input{math_commands.tex}

\usepackage{hyperref}
\usepackage{url}

\title{Formatting Instructions for ICLR 2021 \\ Conference Submissions}

% Authors must not appear in the submitted version. They should be hidden
% as long as the \iclrfinalcopy macro remains commented out below.
% Non-anonymous submissions will be rejected without review.

\author{Antiquus S.~Hippocampus, Natalia Cerebro \& Amelie P. Amygdale \thanks{ Use footnote for providing further information
about author (webpage, alternative address)---\emph{not} for acknowledging
funding agencies.  Funding acknowledgements go at the end of the paper.} \\
Department of Computer Science\\
Cranberry-Lemon University\\
Pittsburgh, PA 15213, USA \\
\texttt{\{hippo,brain,jen\}@cs.cranberry-lemon.edu} \\
\And
Ji Q. Ren \& Yevgeny LeNet \\
Department of Computational Neuroscience \\
University of the Witwatersrand \\
Joburg, South Africa \\
\texttt{\{robot,net\}@wits.ac.za} \\
\AND
Coauthor \\
Affiliation \\
Address \\
\texttt{email}
}

% The \author macro works with any number of authors. There are two commands
% used to separate the names and addresses of multiple authors: \And and \AND.
%
% Using \And between authors leaves it to \LaTeX{} to determine where to break
% the lines. Using \AND forces a linebreak at that point. So, if \LaTeX{}
% puts 3 of 4 authors names on the first line, and the last on the second
% line, try using \AND instead of \And before the third author name.

%\iclrfinalcopy % Uncomment for camera-ready version, but NOT for submission.
\begin{document}

\maketitle

\begin{abstract}
The abstract paragraph should be indented 1/2~inch (3~picas) on both left and
right-hand margins. Use 10~point type, with a vertical spacing of 11~points.
The word \textsc{Abstract} must be centered, in small caps, and in point size 12. Two
line spaces precede the abstract. The abstract must be limited to one
paragraph.
\end{abstract}

\section{Submission of conference papers to ICLR 2021}

ICLR requires electronic submissions, processed by
\url{https://openreview.net/}. See ICLR's website for more instructions.

If your paper is ultimately accepted, the statement {\tt
  {\textbackslash}iclrfinalcopy} should be inserted to adjust the
format to the camera ready requirements.

The format for the submissions is a variant of the NeurIPS format.
Please read carefully the instructions below, and follow them
faithfully.

\subsection{Style}

Papers to be submitted to ICLR 2021 must be prepared according to the
instructions presented here.

%% Please note that we have introduced automatic line number generation
%% into the style file for \LaTeXe. This is to help reviewers
%% refer to specific lines of the paper when they make their comments. Please do
%% NOT refer to these line numbers in your paper as they will be removed from the
%% style file for the final version of accepted papers.

Authors are required to use the ICLR \LaTeX{} style files obtainable at the
ICLR website. Please make sure you use the current files and
not previous versions. Tweaking the style files may be grounds for rejection.

\subsection{Retrieval of style files}

The style files for ICLR and other conference information are available online at:
\begin{center}
   \url{http://www.iclr.cc/}
\end{center}
The file \verb+iclr2021_conference.pdf+ contains these
instructions and illustrates the
various formatting requirements your ICLR paper must satisfy.
Submissions must be made using \LaTeX{} and the style files
\verb+iclr2021_conference.sty+ and \verb+iclr2021_conference.bst+ (to be used with \LaTeX{}2e). The file
\verb+iclr2021_conference.tex+ may be used as a ``shell'' for writing your paper. All you
have to do is replace the author, title, abstract, and text of the paper with
your own.

The formatting instructions contained in these style files are summarized in
sections \ref{gen_inst}, \ref{headings}, and \ref{others} below.

\section{General formatting instructions}
\label{gen_inst}

The text must be confined within a rectangle 5.5~inches (33~picas) wide and
9~inches (54~picas) long. The left margin is 1.5~inch (9~picas).
Use 10~point type with a vertical spacing of 11~points. Times New Roman is the
preferred typeface throughout. Paragraphs are separated by 1/2~line space,
with no indentation.

Paper title is 17~point, in small caps and left-aligned.
All pages should start at 1~inch (6~picas) from the top of the page.

Authors' names are
set in boldface, and each name is placed above its corresponding
address. The lead author's name is to be listed first, and
the co-authors' names are set to follow. Authors sharing the
same address can be on the same line.

Please pay special attention to the instructions in section \ref{others}
regarding figures, tables, acknowledgments, and references.

There will be a strict upper limit of 8 pages for the main text of the initial submission, with unlimited additional pages for citations. Note that the upper page limit differs from last year!Authors may use as many pages of appendices (after the bibliography) as they wish, but reviewers are not required to read these. During the rebuttal phase and for the camera ready version, authors are allowed one additional page for the main text, for a strict upper limit of 9 pages.

\section{Headings: first level}
\label{headings}

First level headings are in small caps,
flush left and in point size 12. One line space before the first level
heading and 1/2~line space after the first level heading.

\subsection{Headings: second level}

Second level headings are in small caps,
flush left and in point size 10. One line space before the second level
heading and 1/2~line space after the second level heading.

\subsubsection{Headings: third level}

Third level headings are in small caps,
flush left and in point size 10. One line space before the third level
heading and 1/2~line space after the third level heading.

\section{Citations, figures, tables, references}
\label{others}

These instructions apply to everyone, regardless of the formatter being used.

\subsection{Citations within the text}

Citations within the text should be based on the \texttt{natbib} package
and include the authors' last names and year (with the ``et~al.'' construct
for more than two authors). When the authors or the publication are
included in the sentence, the citation should not be in parenthesis using \verb|\citet{}| (as
in ``See \citet{Hinton06} for more information.''). Otherwise, the citation
should be in parenthesis using \verb|\citep{}| (as in ``Deep learning shows promise to make progress
towards AI~\citep{Bengio+chapter2007}.'').

The corresponding references are to be listed in alphabetical order of
authors, in the \textsc{References} section. As to the format of the
references themselves, any style is acceptable as long as it is used
consistently.

\subsection{Footnotes}

Indicate footnotes with a number\footnote{Sample of the first footnote} in the
text. Place the footnotes at the bottom of the page on which they appear.
Precede the footnote with a horizontal rule of 2~inches
(12~picas).\footnote{Sample of the second footnote}

\subsection{Figures}

All artwork must be neat, clean, and legible. Lines should be dark
enough for purposes of reproduction; art work should not be
hand-drawn. The figure number and caption always appear after the
figure. Place one line space before the figure caption, and one line
space after the figure. The figure caption is lower case (except for
first word and proper nouns); figures are numbered consecutively.

Make sure the figure caption does not get separated from the figure.
Leave sufficient space to avoid splitting the figure and figure caption.

You may use color figures.
However, it is best for the
figure captions and the paper body to make sense if the paper is printed
either in black/white or in color.
\begin{figure}[h]
\begin{center}
%\framebox[4.0in]{$\;$}
\fbox{\rule[-.5cm]{0cm}{4cm} \rule[-.5cm]{4cm}{0cm}}
\end{center}
\caption{Sample figure caption.}
\end{figure}

\subsection{Tables}

All tables must be centered, neat, clean and legible. Do not use hand-drawn
tables. The table number and title always appear before the table. See
Table~\ref{sample-table}.

Place one line space before the table title, one line space after the table
title, and one line space after the table. The table title must be lower case
(except for first word and proper nouns); tables are numbered consecutively.

\begin{table}[t]
\caption{Sample table title}
\label{sample-table}
\begin{center}
\begin{tabular}{ll}
\multicolumn{1}{c}{\bf PART}  &\multicolumn{1}{c}{\bf DESCRIPTION}
\\ \hline \\
Dendrite         &Input terminal \\
Axon             &Output terminal \\
Soma             &Cell body (contains cell nucleus) \\
\end{tabular}
\end{center}
\end{table}

\section{Default Notation}

In an attempt to encourage standardized notation, we have included the
notation file from the textbook, \textit{Deep Learning}
\cite{goodfellow2016deep} available at
\url{https://github.com/goodfeli/dlbook_notation/}.  Use of this style
is not required and can be disabled by commenting out
\texttt{math\_commands.tex}.

\centerline{\bf Numbers and Arrays}
\bgroup
\def\arraystretch{1.5}
\begin{tabular}{p{1in}p{3.25in}}
$\displaystyle a$ & A scalar (integer or real)\\
$\displaystyle \va$ & A vector\\
$\displaystyle \mA$ & A matrix\\
$\displaystyle \tA$ & A tensor\\
$\displaystyle \mI_n$ & Identity matrix with $n$ rows and $n$ columns\\
$\displaystyle \mI$ & Identity matrix with dimensionality implied by context\\
$\displaystyle \ve^{(i)}$ & Standard basis vector $[0,\dots,0,1,0,\dots,0]$ with a 1 at position $i$\\
$\displaystyle \text{diag}(\va)$ & A square, diagonal matrix with diagonal entries given by $\va$\\
$\displaystyle \ra$ & A scalar random variable\\
$\displaystyle \rva$ & A vector-valued random variable\\
$\displaystyle \rmA$ & A matrix-valued random variable\\
\end{tabular}
\egroup
\vspace{0.25cm}

\centerline{\bf Sets and Graphs}
\bgroup
\def\arraystretch{1.5}

\begin{tabular}{p{1.25in}p{3.25in}}
$\displaystyle \sA$ & A set\\
$\displaystyle \R$ & The set of real numbers \\
$\displaystyle \{0, 1\}$ & The set containing 0 and 1 \\
$\displaystyle \{0, 1, \dots, n \}$ & The set of all integers between $0$ and $n$\\
$\displaystyle [a, b]$ & The real interval including $a$ and $b$\\
$\displaystyle (a, b]$ & The real interval excluding $a$ but including $b$\\
$\displaystyle \sA \backslash \sB$ & Set subtraction, i.e., the set containing the elements of $\sA$ that are not in $\sB$\\
$\displaystyle \gG$ & A graph\\
$\displaystyle \parents_\gG(\ervx_i)$ & The parents of $\ervx_i$ in $\gG$
\end{tabular}
\vspace{0.25cm}

\centerline{\bf Indexing}
\bgroup
\def\arraystretch{1.5}

\begin{tabular}{p{1.25in}p{3.25in}}
$\displaystyle \eva_i$ & Element $i$ of vector $\va$, with indexing starting at 1 \\
$\displaystyle \eva_{-i}$ & All elements of vector $\va$ except for element $i$ \\
$\displaystyle \emA_{i,j}$ & Element $i, j$ of matrix $\mA$ \\
$\displaystyle \mA_{i, :}$ & Row $i$ of matrix $\mA$ \\
$\displaystyle \mA_{:, i}$ & Column $i$ of matrix $\mA$ \\
$\displaystyle \etA_{i, j, k}$ & Element $(i, j, k)$ of a 3-D tensor $\tA$\\
$\displaystyle \tA_{:, :, i}$ & 2-D slice of a 3-D tensor\\
$\displaystyle \erva_i$ & Element $i$ of the random vector $\rva$ \\
\end{tabular}
\egroup
\vspace{0.25cm}

\centerline{\bf Calculus}
\bgroup
\def\arraystretch{1.5}
\begin{tabular}{p{1.25in}p{3.25in}}
% NOTE: the [2ex] on the next line adds extra height to that row of the table.
% Without that command, the fraction on the first line is too tall and collides
% with the fraction on the second line.
$\displaystyle\frac{d y} {d x}$ & Derivative of $y$ with respect to $x$\\ [2ex]
$\displaystyle \frac{\partial y} {\partial x} $ & Partial derivative of $y$ with respect to $x$ \\
$\displaystyle \nabla_\vx y $ & Gradient of $y$ with respect to $\vx$ \\
$\displaystyle \nabla_\mX y $ & Matrix derivatives of $y$ with respect to $\mX$ \\
$\displaystyle \nabla_\tX y $ & Tensor containing derivatives of $y$ with respect to $\tX$ \\
$\displaystyle \frac{\partial f}{\partial \vx} $ & Jacobian matrix $\mJ \in \R^{m\times n}$ of $f: \R^n \rightarrow \R^m$\\
$\displaystyle \nabla_\vx^2 f(\vx)\text{ or }\mH( f)(\vx)$ & The Hessian matrix of $f$ at input point $\vx$\\
$\displaystyle \int f(\vx) d\vx $ & Definite integral over the entire domain of $\vx$ \\
$\displaystyle \int_\sS f(\vx) d\vx$ & Definite integral with respect to $\vx$ over the set $\sS$ \\
\end{tabular}
\egroup
\vspace{0.25cm}

\centerline{\bf Probability and Information Theory}
\bgroup
\def\arraystretch{1.5}
\begin{tabular}{p{1.25in}p{3.25in}}
$\displaystyle P(\ra)$ & A probability distribution over a discrete variable\\
$\displaystyle p(\ra)$ & A probability distribution over a continuous variable, or over
a variable whose type has not been specified\\
$\displaystyle \ra \sim P$ & Random variable $\ra$ has distribution $P$\\% so thing on left of \sim should always be a random variable, with name beginning with \r
$\displaystyle  \E_{\rx\sim P} [ f(x) ]\text{ or } \E f(x)$ & Expectation of $f(x)$ with respect to $P(\rx)$ \\
$\displaystyle \Var(f(x)) $ &  Variance of $f(x)$ under $P(\rx)$ \\
$\displaystyle \Cov(f(x),g(x)) $ & Covariance of $f(x)$ and $g(x)$ under $P(\rx)$\\
$\displaystyle H(\rx) $ & Shannon entropy of the random variable $\rx$\\
$\displaystyle \KL ( P \Vert Q ) $ & Kullback-Leibler divergence of P and Q \\
$\displaystyle \mathcal{N} ( \vx ; \vmu , \mSigma)$ & Gaussian distribution %
over $\vx$ with mean $\vmu$ and covariance $\mSigma$ \\
\end{tabular}
\egroup
\vspace{0.25cm}

\centerline{\bf Functions}
\bgroup
\def\arraystretch{1.5}
\begin{tabular}{p{1.25in}p{3.25in}}
$\displaystyle f: \sA \rightarrow \sB$ & The function $f$ with domain $\sA$ and range $\sB$\\
$\displaystyle f \circ g $ & Composition of the functions $f$ and $g$ \\
  $\displaystyle f(\vx ; \vtheta) $ & A function of $\vx$ parametrized by $\vtheta$.
  (Sometimes we write $f(\vx)$ and omit the argument $\vtheta$ to lighten notation) \\
$\displaystyle \log x$ & Natural logarithm of $x$ \\
$\displaystyle \sigma(x)$ & Logistic sigmoid, $\displaystyle \frac{1} {1 + \exp(-x)}$ \\
$\displaystyle \zeta(x)$ & Softplus, $\log(1 + \exp(x))$ \\
$\displaystyle || \vx ||_p $ & $\normlp$ norm of $\vx$ \\
$\displaystyle || \vx || $ & $\normltwo$ norm of $\vx$ \\
$\displaystyle x^+$ & Positive part of $x$, i.e., $\max(0,x)$\\
$\displaystyle \1_\mathrm{condition}$ & is 1 if the condition is true, 0 otherwise\\
\end{tabular}
\egroup
\vspace{0.25cm}

\section{Final instructions}
Do not change any aspects of the formatting parameters in the style files.
In particular, do not modify the width or length of the rectangle the text
should fit into, and do not change font sizes (except perhaps in the
\textsc{References} section; see below). Please note that pages should be
numbered.

\section{Preparing PostScript or PDF files}

Please prepare PostScript or PDF files with paper size ``US Letter'', and
not, for example, ``A4''. The -t
letter option on dvips will produce US Letter files.

Consider directly generating PDF files using \verb+pdflatex+
(especially if you are a MiKTeX user).
PDF figures must be substituted for EPS figures, however.

Otherwise, please generate your PostScript and PDF files with the following commands:
\begin{verbatim}
dvips mypaper.dvi -t letter -Ppdf -G0 -o mypaper.ps
ps2pdf mypaper.ps mypaper.pdf
\end{verbatim}

\subsection{Margins in LaTeX}

Most of the margin problems come from figures positioned by hand using
\verb+\special+ or other commands. We suggest using the command
\verb+\includegraphics+
from the graphicx package. Always specify the figure width as a multiple of
the line width as in the example below using .eps graphics
\begin{verbatim}
   \usepackage[dvips]{graphicx} ...
   \includegraphics[width=0.8\linewidth]{myfile.eps}
\end{verbatim}
or % Apr 2009 addition
\begin{verbatim}
   \usepackage[pdftex]{graphicx} ...
   \includegraphics[width=0.8\linewidth]{myfile.pdf}
\end{verbatim}
for .pdf graphics.
See section~4.4 in the graphics bundle documentation (\url{http://www.ctan.org/tex-archive/macros/latex/required/graphics/grfguide.ps})

A number of width problems arise when LaTeX cannot properly hyphenate a
line. Please give LaTeX hyphenation hints using the \verb+\-+ command.

\subsubsection*{Author Contributions}
If you'd like to, you may include  a section for author contributions as is done
in many journals. This is optional and at the discretion of the authors.

\subsubsection*{Acknowledgments}
Use unnumbered third level headings for the acknowledgments. All
acknowledgments, including those to funding agencies, go at the end of the paper.

\bibliography{iclr2021_conference}
\bibliographystyle{iclr2021_conference}

\appendix
\section{Appendix}
You may include other additional sections here.

\end{document}
